# Supplementary material for: Prediction of deformed halo nuclei $^{43,45}$Si from multiple criteria based on structure and reaction analyses
Source: arXiv:2512.14545 source file (2026-04-02)
Supplement: Supplementary file 1 [file Supplementary_material.pdf]

# Supplemental Material for Prediction of deformed halo nuclei $^{43,45}\text{Si}$ from multiple criteria based on structure and reaction analyses

C. Pan (潘琮)<sup>a</sup>, J. L. An (安嘉琳)<sup>b</sup>, P. Ring<sup>c,d</sup>, X. H. Wu (吴鑫辉)<sup>e</sup>, P. Papakonstantinou<sup>f</sup>, M.-H. Mun<sup>g</sup>, Y. Kim<sup>h</sup>, S. S. Zhang (张时声)<sup>b</sup>, K. Y. Zhang (张开元)<sup>i</sup>

<sup>a</sup>Department of Physics, Anhui Normal University, Wuhu 241000, China

<sup>b</sup>School of Physics, Beihang University, Beijing 100191, China

<sup>c</sup>Physik-Department der Technischen Universität München, D-85748 Garching, Germany

<sup>d</sup>State Key Laboratory of Nuclear Physics and Technology, School of Physics, Peking University, Beijing 100871, China

<sup>e</sup>Department of Physics, Fuzhou University, Fuzhou 350108, Fujian, China

<sup>f</sup>Institute for Rare Isotope Science, Institute for Basic Science, Daejeon 34000, Republic of Korea

<sup>g</sup>Department of Physics, Kyungpook National University, Daegu 41566, Republic of Korea

<sup>h</sup>Center for Exotic Nuclear Studies, Institute for Basic Science, Daejeon 34126, Republic of Korea

<sup>i</sup>National Key Laboratory of Neutron Science and Technology, Institute of Nuclear Physics and Chemistry, China Academy of Engineering Physics, Mianyang, Sichuan 621900, China

## 1. Dependence on pairing parameters

In the particle-particle channel, the density-dependent zero-range pairing force is adopted in the DRHBc calculations for silicon isotopes. The pairing parameters, *i.e.*, the pairing cutoff (pairing window)  $E_{\text{cut}}^{\text{qp}} = 100$  MeV and the pairing strength  $V_0 = 325$  MeV fm<sup>3</sup>, are the same as those in the DRHBc mass table calculations, which were determined by reproducing the experimental odd-even mass differences for Ca and Pb isotopes [1].

In Ref. [2], it is shown that beyond the region where the pairing parameters are adjusted, different  $E_{\text{cut}}^{\text{qp}}$  values might produce inconsistent results. Therefore, here we examine whether changing pairing cutoff influences the halo phenomenon. Taking three cutoff values  $E_{\text{cut}}^{\text{qp}} = 100, 80$  and 60 MeV as examples, by minimizing the rms deviation of calculated odd-even mass differences from available data of neutron-rich Si isotopes, the sets  $(E_{\text{cut}}^{\text{qp}}, V_0) = (100, 350), (80, 380)$  and  $(60, 420)$  are obtained.

Figure S1 shows the one-neutron separation energies for neutron-rich silicon isotopes calculated using these pairing parameters, which are found essentially consistent with the (100, 325)-results in the main text, particularly for  $^{43,45}\text{Si}$ .

Figure S2 shows the neutron density distributions for  $^{43,45}\text{Si}$  calculated using these new pairing parameters. The new results again coincide with the original ones—all are significantly larger than those of their even-even neighbors at large  $r$ . It is also noted that the results calculated with new pairing parameter sets exhibit slightly more extended distributions, which can be partially attributed to their smaller  $S_{1n}$  values shown in Fig. S1. Consequently, the prediction of neutron halos in  $^{43,45}\text{Si}$  is independent of the pairing cutoff.

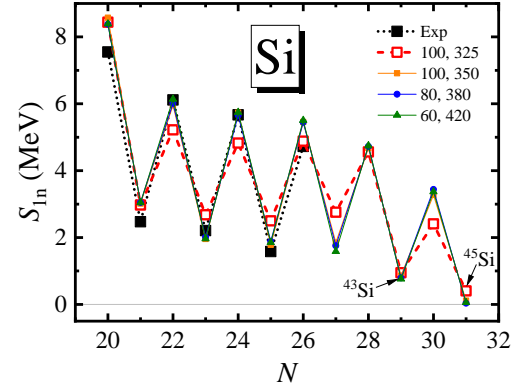

Figure S1: One-neutron separation energy  $S_{1n}$  as a function of neutron number  $N$  for neutron-rich silicon isotopes, calculated by DRHBc with different pairing parameters  $(E_{\text{cut}}^{\text{qp}}, V_0)$ . The units of  $(E_{\text{cut}}^{\text{qp}}, V_0)$  are (MeV, MeV fm<sup>3</sup>). The available experimental data from AME2020 [3] are shown for comparison.

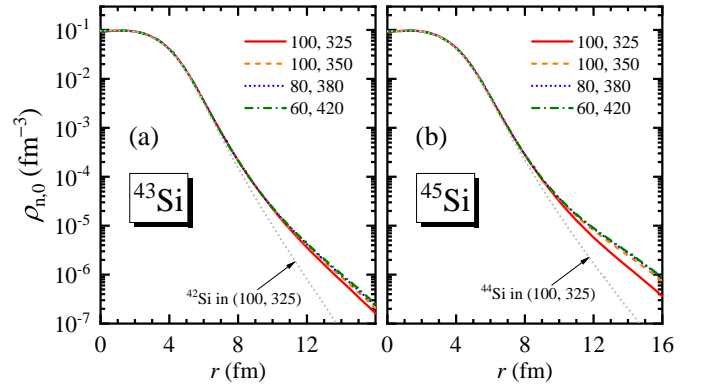

Figure S2: Angle average neutron density distributions for  $^{43}\text{Si}$  (a) and  $^{45}\text{Si}$  (b), calculated by DRHBc with different pairing parameters  $(E_{\text{cut}}^{\text{qp}}, V_0)$ . The units of  $(E_{\text{cut}}^{\text{qp}}, V_0)$  are (MeV, MeV fm<sup>3</sup>). The densities of even-even neighbors are shown for comparison.

## 2. Dependence on density functional

In the particle-hole channel, four relativistic density functionals PC-PK1 [4], PC-L3R [5], NL3\* [6], and NL-SH [7] are adopted in this work. The corresponding  $S_{1n}$  values have been compared in Fig. 1 of the main text.

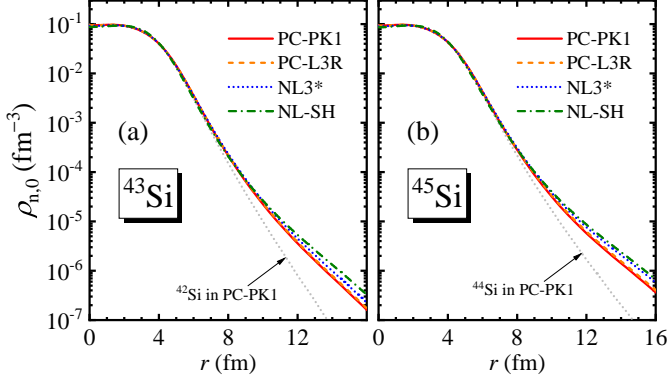

Figure S3: Angle average neutron density distributions for <sup>43</sup>Si (a) and <sup>45</sup>Si (b), calculated by DRHBc with different density functionals. The densities of even-even neighbors are shown for comparison.

Figure S3 shows the neutron density distributions of <sup>43,45</sup>Si calculated with these density functionals. All the employed functionals yield results consistent with each other in both trend and magnitude. Therefore, the prediction of neutron halos in <sup>43,45</sup>Si is independent of the choice of density functional.

## 3. Discussion on <sup>41</sup>Si

In the main text, the reaction analysis shows halo-like behaviors for <sup>41</sup>Si in Fig. 7, while it is not supported as a halo nucleus from the structure perspective. This is because the Glauber-model calculation assumes a “core +  $n$ ” structure, which is not well established for <sup>41</sup>Si, as demonstrated below.

Figure S4 shows the single-neutron levels around the continuum threshold for <sup>41</sup>Si. It can be found that the valence-neutron  $1/2^-$  orbital of <sup>41</sup>Si is not as loosely bound as those in <sup>43,45</sup>Si (shown in Fig. 4 of the main text). Meanwhile, it lies close to the  $3/2^-$  orbital, with no sizable gap formed between the valence orbital and the core orbitals. This is in sharp contrast to the cases of the predicted halo nuclei <sup>43,45</sup>Si, where the halo orbital is well decoupled in energy from the core orbitals [Fig. 4 of the main text].

Figure S5 shows the densities of individual single-neutron orbitals in <sup>41</sup>Si, in comparison with those in <sup>43</sup>Si. For <sup>41</sup>Si in Fig. S5(a), the density of the valence-neutron orbital  $1/2^-$  is smaller than that of the  $3/2^-$  orbital. Consequently, its contribution to the total neutron density is lower than that from the  $3/2^-$  orbital. This is clearly inconsistent with the classic picture of a halo nucleus, in which the valence nucleon(s) dominates the density in the asymptotic region. In contrast, for <sup>43</sup>Si in Fig. S5(b), the valence-neutron orbital is well decoupled in spatial distribution from the core

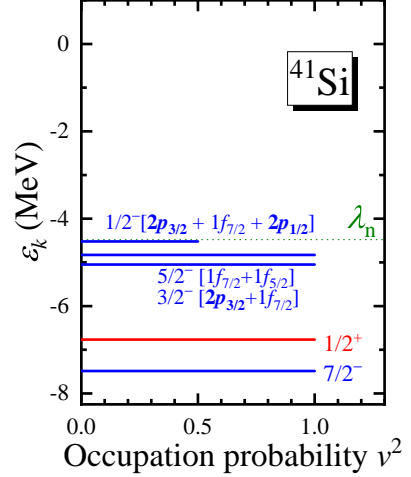

Figure S4: Single-neutron levels around the continuum threshold in the canonical basis for <sup>41</sup>Si versus the occupation probability  $v^2$  in the DRHBc calculations. The levels are labeled by the quantum numbers  $m^\pi$ , and the main components in the DWS basis are given for the levels above -6 MeV. The Fermi energy  $\lambda_n$  is shown by a dotted line.

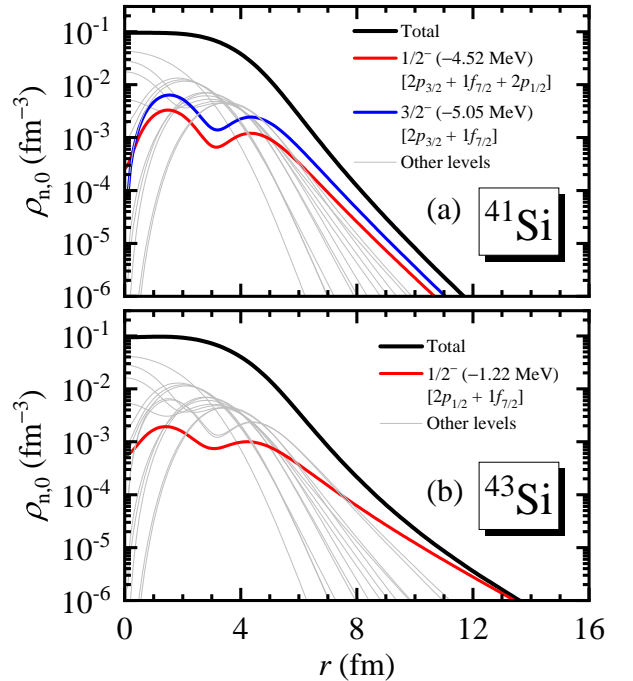

Figure S5: Angle-averaged densities of individual single-neutron orbitals in <sup>41</sup>Si (a) and <sup>43</sup>Si (b), along with the total neutron density, plotted as functions of the radial coordinate  $r$ .

orbitals, forming an extended tail of the neutron density. Therefore, from the structure perspective, <sup>41</sup>Si is not suggested as a halo nucleus and does not exhibit a “core +  $n$ ” structure.

## References

- [1] K. Zhang, M.-K. Cheoun, Y.-B. Choi, P. S. Chong, J. Dong, L. Geng, E. Ha, X. He, C. Heo, M. C. Ho,

- E. J. In, S. Kim, Y. Kim, C.-H. Lee, J. Lee, Z. Li, T. Luo, J. Meng, M.-H. Mun, Z. Niu, C. Pan, P. Papakonstantinou, X. Shang, C. Shen, G. Shen, W. Sun, X.-X. Sun, C. K. Tam, Thaivayongnou, C. Wang, S. H. Wong, X. Xia, Y. Yan, R. W.-Y. Yeung, T. C. Yiu, S. Zhang, W. Zhang, S.-G. Zhou, Deformed relativistic Hartree-Bogoliubov theory in continuum with a point-coupling functional: Examples of even-even Nd isotopes, *Phys. Rev. C* 102 (2020) 024314. doi:10.1103/PhysRevC.102.024314.
- [2] S. Karatzikos, A. Afanasjev, G. Lalazissis, P. Ring, The fission barriers in actinides and superheavy nuclei in covariant density functional theory, *Phys. Lett. B* 689 (2) (2010) 72–81. doi:<https://doi.org/10.1016/j.physletb.2010.04.045>.
- [3] M. Wang, W. J. Huang, F. G. Kondev, G. Audi, S. Naimi, The AME 2020 atomic mass evaluation (II). tables, graphs and references, *Chin. Phys. C* 45 (3) (2021) 030003. doi:10.1088/1674-1137/abddaf.
- [4] P. W. Zhao, Z. P. Li, J. M. Yao, J. Meng, New parametrization for the nuclear covariant energy density functional with a point-coupling interaction, *Phys. Rev. C* 82 (2010) 054319. doi:10.1103/PhysRevC.82.054319.
- [5] Z. X. Liu, Y. H. Lam, N. Lu, P. Ring, The optimized point-coupling interaction for the relativistic energy density functional of hartree-bogoliubov approach quantifying the nuclear bulk properties, *Phys. Lett. B* 842 (2023) 137946. doi:<https://doi.org/10.1016/j.physletb.2023.137946>.
- [6] G. Lalazissis, S. Karatzikos, R. Fossion, D. P. Arteaga, A. Afanasjev, P. Ring, The effective force nl3 revisited, *Phys. Lett. B* 671 (1) (2009) 36–41. doi:<https://doi.org/10.1016/j.physletb.2008.11.070>.
- [7] M. Sharma, M. Nagarajan, P. Ring, Rho meson coupling in the relativistic mean field theory and description of exotic nuclei, *Phys. Lett. B* 312 (4) (1993) 377–381. doi:[https://doi.org/10.1016/0370-2693\(93\)90970-S](https://doi.org/10.1016/0370-2693(93)90970-S).
